# Supplementary material for: Density Distribution-based Learning Framework for Addressing Online Continual Learning Challenges
Source: arXiv:2311.13623 source file (2023-11-22)
Supplement: Supplementary file 1 [file X_suppl.tex]

\clearpage
\setcounter{page}{1}
\maketitlesupplementary

\section*{A. The Proof Of The Bias and Variance}

The bias and variance of the GKDE for a scalar bandwidth $h$ in low dimensional space is:

\begin{align}
	\mathrm{Bias}[\hat{f}(z;h)]&=\frac{1}{2}\mu_2(K)f''(z)h^2+o(h^2),\tag{1}\\
	\mathbb{V}\mathrm{ar}[\hat{f}(z;h)]&=\frac{R(K)}{nh}f(z)+o((nh)^{-1}),\tag{2}
\end{align}
where $R(f):=\int f(z)^2\,\mathrm{d}z$ and $\mu_2(K):=\int z^2 K(z)\,\mathrm{d}z$. 
\\ \hspace*{\fill} \\
To prove the above formula, we need the convolution between two real functions:

\begin{align}
	(f*g)(z):=\int f(z-t)g(t)\,\mathrm{d}y=(g*f)(z).\tag{3}
\end{align}

The expectation of $\hat{f}(x;h)$ can be expressed as:
\begin{align}
	\mathbb{E}[\hat{f}(z;h)]&=\lim_{n \to +\infty} \frac{1}{n}\sum_{i=1}^n\mathbb{E}[K_h(z-Z_i)]\nonumber\\
	&=\int K_h(z-Z)f(Z)\,\mathrm{d}Z\nonumber.\tag{4}
\end{align}

By changing the variable, $t=\frac{z-Z}{h},Z=z-ht,\mathrm{d}Z=-h\,\mathrm{d}t$:

\begin{align}
	\mathbb{E}[\hat{f}(z;h)] &=\int K(t)f(z-ht)\,\mathrm{d}t.\tag{5}
\end{align}

The second-order Taylor expansion of $f(z-ht)$ given $h\to0$ leads to:
\begin{align}
	f(z-ht)=&\,f(z)-f'(z)ht+\frac{f''(z)}{2}h^2t^2\nonumber\\
	&+o(h^2t^2). \tag{6}
\end{align}

Substituting Eq.6 in Eq.5 gives:

\begin{align*}
	\int K(t)&f(z-ht)\,\mathrm{d}t\\
	=&\,\int K(t)\Big\{f(z)-f'(z)ht+\frac{f''(z)}{2}h^2t^2\\
	&+o(h^2t^2)\Big\}\,\mathrm{d}t\\
	=&\,f(z)+\frac{1}{2}\mu_2(K)f''(z)h^2+o(h^2),\tag{7}
\end{align*}
where $K(t)$ is a symmetric density kernel with a mean of 0 and the cumulative distribution of $K(t)$ is 1, which leads to the second equation in Eq.7. The notation $\mu_2(K):=\int z^2 K(z),\mathrm{d}z$ is simply used to make the formula more concise. From Eq.7, we can obtain:

\begin{align*}
	\mathrm{Bias}[\hat{f}(z;h)]&=\mathbb{E}[\hat{f}(z;h)] - f(z) \\
	&=\frac{1}{2}\mu_2(K)f''(z)h^2+o(h^2),\tag{8}\\
\end{align*}

For a high dimensional $\mathbf{z}$ and bandwidth matrix $\mathbf{H}$, the expectation is:
\begin{align*}
	\mathbb{E}[\hat{f}(\mathbf{z};\mathbf{H})]&=\int K_\mathbf{H}(\mathbf{z}-\mathbf{Z})f(\mathbf{Z})\,\mathrm{d}\mathbf{Z}\\
	&=\int K(\mathbf{t})f(\mathbf{z}-\mathbf{H}^{1/2}\mathbf{t})\,\mathrm{d}\mathbf{t}.\tag{9}
\end{align*}

The variable in Eq.5 is replaced by its high dimensional version,  $\mathbf{t}=\mathbf{H}^{-1/2}(\mathbf{z}-\mathbf{Z}),\mathbf{Z}=\mathbf{z}-\mathbf{H}^{1/2}\mathbf{t}, \mathrm{d}\mathbf{Z}=-|\mathbf{H}|^{1/2}\,\mathrm{d}\mathbf{t}$. The Taylor expansion for $f(\mathbf{z}-\mathbf{H}^{1/2}\mathbf{t})$ can also be used to obtain:
\begin{align}
	\mathrm{Bias}[\hat{f}(\mathbf{z};\mathbf{H})]&=\frac{1}{2}\mu_2(K)(\mathrm{D}^{\otimes2}f(\mathbf{z}))'\mathrm{vec}\,\mathbf{H}+o(\|\mathrm{vec}\,\mathbf{H}\|),\tag{10}
\end{align}
which ends the conclusion of the bias of the GKDE. By using a change of variables and employing a first-order Taylor expansion, we can derive the variance of the GKDE as follows:

\begin{align}
	\mathbb{E}[K_h^2(z-Z)]&=\frac{1}{h}\int K^2(t)f(z-ht)\,\mathrm{d}t\nonumber\\
	&=\frac{1}{h}\int K^2(t)\left\{f(z)+O(ht)\right\}\,\mathrm{d}t\nonumber\\
	&=\frac{R(K)}{h}f(z)+O(1). \tag{11}
\end{align}

Then the variance of GKDE can be expressed as:

\begin{align}
	\mathbb{V}\mathrm{ar}[\hat{f}(z;h)]&=\frac{1}{n^2}\sum_{i=1}^n\mathbb{V}\mathrm{ar}[K_h(z-Z_i)]\nonumber\\
	&=\frac{1}{n}\left\{\mathbb{E}[K_h^2(z-Z)]-\mathbb{E}[K_h(z-Z)]^2\right\}\nonumber\\
	&=\frac{1}{n}\left\{\frac{R(K)}{h}f(x)+O(1)-O(1)\right\}\nonumber\\
	&=\frac{R(K)}{nh}f(x)+O(n^{-1})\nonumber\\
	&=\frac{R(K)}{nh}f(x)+o((nh)^{-1}),	 \tag{12}
\end{align}
where $R(f):=\int f(z)^2\,\mathrm{d}z$. The Eq.12 is derived from Eq.11 and Eq.5 and the fact that $n^{-1}=o((nh)^{-1})$. For high-dimensional $\mathbf{z}$ and bandwidth matrix $\mathbf{H}$, the same conclusion holds, namely:

\begin{align}
	\mathbb{V}\mathrm{ar}[\hat{f}(\mathbf{z};\mathbf{H})]&=\frac{R(K)}{n|\mathbf{H}|^{1/2}}f(\mathbf{z})+o((n|\mathbf{H}|^{1/2})^{-1}).\tag{13}
\end{align}

\section*{B. Task Incremental Experiment on TinyImageNet}

We conducted sequential execution of 100 tasks in TinyImageNet, with each task consisting of 2 classes. In Figure 7, we present the average accuracy achieved by the GKDE based on ResNet18 and VIT. These tasks pose a greater challenge due to the significantly larger number of tasks compared to other datasets. Thanks to the integrated framework of Model Bank and TP-WP classification process, our method effectively avoids the DF issue. However, the models based on ResNet18 and VIT exhibit varying accuracies due to the differences in their feature extraction abilities provided by the respective backbones.

\begin{figure}
	\label{TinyImageNet}
	\centering
	\includegraphics[width=2.9 in,height=2.6 in]{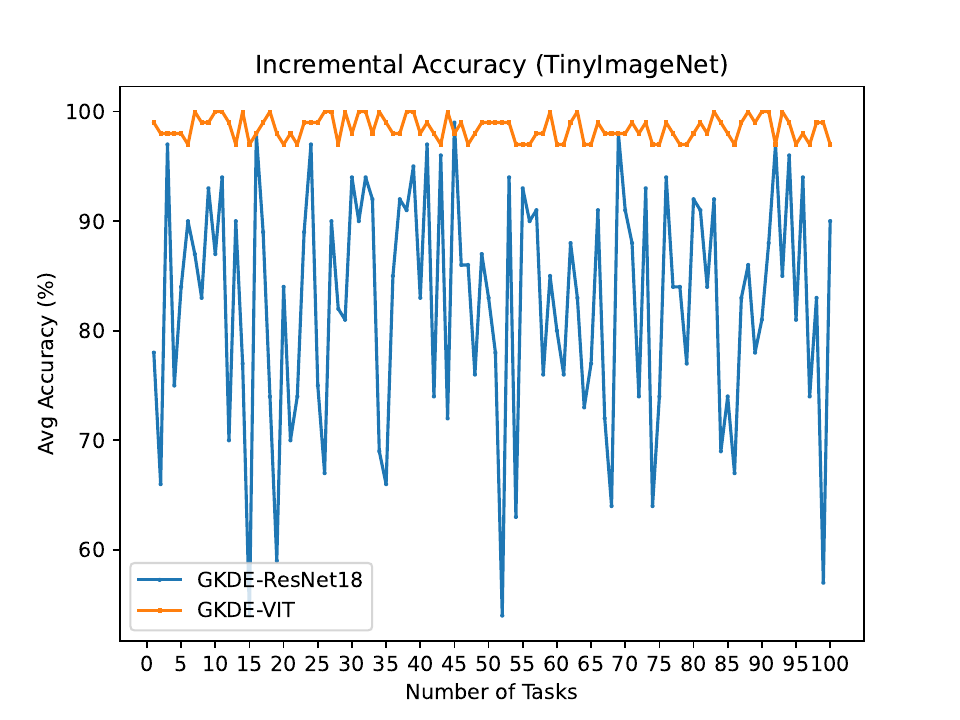}
	\caption{Task Incremental Experiment on TinyImageNet. The GKDE based on ResNet18 achieves varying accuracies on the 100 tasks. the VIT backbone consistently achieves accuracy of over 98\%. }
\end{figure}

Figure 7 shows that the GKDE based on ResNet18 achieves varying accuracies on the 100 tasks of TinyImageNet, indicating differences in task complexity. For instance, the method achieves accuracy above 98\% on specific tasks, while falling below 60\% on others. We can conclude that the performance improvement is limited by the backbone features extracted. On the other hand, the VIT backbone, known for its excellent feature extraction ability, consistently achieves accuracy of over 98\%.

\section*{C. Memory Usage Analysis of the GKDE}
For each task, there are two components that contribute to memory usage: the feature extraction backbone and the PDF. In this section, we will compare the memory usage of both components for each backbone and each setting.

\begin{table}[htbp]
	\centering
	\caption{Dataset Comparison}
	\label{tab:dataset}
	\begin{tabular}{cccccc}
		\toprule
		Dataset & ResNet18 & VIT & PDF \\
		\midrule
		Cifar10 & 44.9M & 346.4M & 274k \\
		Cifar100 & 44.9M & 346.4M & 836k \\
		TinyImageNet & 44.9M & 346.4M & 836k\\
		\bottomrule
	\end{tabular}
\end{table}

As shown in Tab.2, each task on different datasets requires storing one backbone and one Probability Density Function (PDF) on disk. During the testing phase, these stored backbones and PDFs need to be loaded into memory for making predictions. The size of the PDF is negligible compared to the backbones. For example, ResNet18 requires 44.9MB, while the PDF (with 32 dimensions and 500 samples) is only 274KB. However, in the case of TinyImageNet, each task requires 346.4MB for the backbone and 836KB for the PDF, which is memory inefficient. To address this issue, an efficient Model Bank design should be implemented to manage the task models based on the hit rate of each stored task model. In our experiments, the models with pre-defined tasks are all stored on disks, and during the testing phase, each model is read into memory for making TP and WP predictions. Further exploration is needed to optimize the storage of backbone models in future works.
